# Supplementary material for: DecentNeRFs: Decentralized Neural Radiance Fields from Crowdsourced Images
Source: arXiv:2403.13199 source file (2024-03-28)
Supplement: Supplementary file 1 [file X_suppl.tex]

\clearpage
\setcounter{page}{1}
% \end{comment}
% \begin{NoHyper}

%%
%% If your work has an appendix, this is the place to put it.
%\renewcommand{\thesection}{S\arabic{section}}

\begin{center}
{\large Supplementary Material\\
\textbf{DecentNeRFs: Decentralized Neural Radiance Fields\\ from Crowdsourced Images}}
\vspace{1em}
\end{center}

\appendix
% \maketitlesupplementary

% \section{Rationale}
% \label{sec:rationale}
% % 
% Having the supplementary compiled together with the main paper means that:
% % 
% \begin{itemize}
% \item The supplementary can back-reference sections of the main paper, for example, we can refer to \cref{sec:intro};
% \item The main paper can forward reference sub-sections within the supplementary explicitly (e.g. referring to a particular experiment); 
% \item When submitted to arXiv, the supplementary will already included at the end of the paper.
% \end{itemize}
% % 
% To split the supplementary pages from the main paper, you can use \href{https://support.apple.com/en-ca/guide/preview/prvw11793/mac#:~:text=Delete%20a%20page%20from%20a,or%20choose%20Edit%20%3E%20Delete).}{Preview (on macOS)}, \href{https://www.adobe.com/acrobat/how-to/delete-pages-from-pdf.html#:~:text=Choose%20%E2%80%9CTools%E2%80%9D%20%3E%20%E2%80%9COrganize,or%20pages%20from%20the%20file.}{Adobe Acrobat} (on all OSs), as well as \href{https://superuser.com/questions/517986/is-it-possible-to-delete-some-pages-of-a-pdf-document}{command line tools}.

% \section{Privacy Leakage for non-overlapping views}
% \label{sec:privacy leakage}

% \subsection{Averaging for overlapping views}
\section{Supplementary Video}
In the supplementary material, we have included a video that visually illustrates the key features and results of our DecentNeRF approach, providing compelling evidence to support our claims. This video serves as a powerful complement to the written content, offering a more immersive and intuitive understanding of our work.

% \subsection{Varying Images per User}

% \section{why don't we just mask everything?}
% Explicitly masking everything would fail

% \section{fraction of data being used for training for phototoursim data}

% \section{DecentNeRF Additional Evaluations}
% In this section, we evaluate the reconstruction performance of DecentNeRF with varying degrees of occlusion.

% \subsection{Varying Occlusion}
% \begin{table}[ht]
% \centering
% \scalebox{1.0}{\hspace{1pt}
% \begin{tabularx}{\linewidth}{l|c|c|c}
% Lego People & PSNR \uparrow & SSIM \uparrow & LPIPS \downarrow \\ \hline
% 1 & 29.25 &	0.97 & 0.0383 \\ \hline
% 6 & 26.25 &	0.92 & 0.0652 \\ \hline
% 12 & 22.80 & 0.89 & 0.1120 \\ \hline

% \end{tabularx}}
% \caption{Varying the number of Lego people as a proxy for occlusion}

% \label{tab:varying_occ}
% \end{table}

\section{Compute Comparisons}
\label{sec:sup_compute}
\subsection{Complexity Comparison}
\noindent\textbf{Offline Communication and Computation} For each round of aggregation, each user prepares offline coded random masks and distributes them to the users.

\noindent \textbf{Reconstruction} Decoding process to reconstruct the weighted average of the obfuscated weights sent by the users. 

\noindent \textbf{Online Communication} Sending and receiving of obfuscated and receiving of weights and gradients. 

In Table \ref{tab:complexity_comparison} we note that DecentNeRF has the same server complexity as FedAvg \cite{mcmahan2017communication} at the cost of incurring more user complexity. 

\begin{table}[ht]
\centering
\vspace{20 pt}
\begin{tabularx}{\columnwidth}{l|X|X}
\hline
& \textbf{FedNeRF} & \textbf{DecentNeRF} \\
\hline
offline comm. (U) & \(O(sN)\) & \(O(sN^2 + dN)\) \\
\hline
offline comp. (U) & \(O(dN + sN^2)\) & \(O(dN^2)\) \\
\hline
online comm. (U) & \(O(d + sN)\) & \(O(dN + sN^2)\) \\
\hline
online comm. (S) & \(O(dN + sN^2)\) & \(O(dN + sN^2)\) \\
\hline
online comp. (U) & \(O(d)\) & \(O(dN^2)\) \\
\hline
reconstruction (S) & \(O(dN^2)\) & \(O(dN^2)\) \\
\hline
\end{tabularx}
\vspace{8 pt}
\caption{Complexity comparison between FedAvg \cite{mcmahan2017communication} and DecentNeRF. In terms of server computing, DecentNeRF has the same complexity but utilizes higher user computing. Here \( \mathbf{N} \) is the total number of users, \( \mathbf{d} \) is the model size, and \( \mathbf{s} \) is the length of the secret keys as the seeds for Pseudo-Random Generator (\( \mathbf{s} \ll \mathbf{d} \)). U is for User and S is for Server} 
\label{tab:complexity_comparison}
\end{table}

\subsection{Server Compute}
Here we show how server compute (in terms of FLOPs) is estimated for one of the example blender scenes in Table \ref{tab:blender_baseline}.  

\noindent \textbf{NeRF-W}: For rendering one batch of rays (4096), SOTA NeRF algorithms such as the one by Müller et al. \cite{muller2022instant} take about \( \approx 350 \times 10^6 \) FLOPs (approximately \( 10^4 \) times faster than vanilla NeRF \cite{nerf}). For the Lego dataset, which has 100 images of size \( 800 \times 800 \) pixels, this leads to 12,500 batches for one epoch, resulting in a total cost of approximately \( 4.8 \times 10^{12} \) FLOPs per epoch. Training the scene for 30 epochs requires around \( 130 \times 10^{12} \) FLOPs of computing on the server. Here, we note that the compute cost for the server scales with the number of pixels in the complete dataset.

\noindent \textbf{FedNeRF}: It requires the addition of 20 (number of users) Global MLP weights per round, each MLP having around 1 million parameters. 1 addition is equivalent to 1 FLOP. For 30 federation rounds, the total computation cost at the server is approximately \( 0.6 \times 10^9 \) FLOPs. In a decentralized setting, we note that the computing cost scales by number of Users.

\noindent \textbf{DecentNeRF}: In addition to the aggregation of user weights, similar to FedNeRF, the server computes the aggregate of gradients, which incurs the same computational cost as the aggregation of weights in FedNeRF, approximately \( 0.6 \times 10^9 \) FLOPs. The computation of the dot product between each user's weights and the aggregated sum of gradients incurs an additional \( 1.2 \times 10^9 \) FLOPs (accounting for parameter-wise multiplication and summation). For the reconstruction cost, we utilize Secure Aggregation (SecAgg+) \cite{bell2020secure}, which has \( O(dN\log N) \) complexity for the previous 4 computations, incurring an additional \( 3 \times 10^9 \) FLOPs.

\section{Implementation Details}
\label{sec:sup_implementation}
\textbf{Training Details}
We use a PyTorch implementation of NeRF-W \cite{nerf_pl_nerfw} for centralized evaluation, which is a variant of vanilla NeRF \cite{nerf}. As shown in Figure~\ref{fig:method}, the Global Radiance Field $\mathbf{G}$, consists of eight layers with 256 hidden units each, followed by an MLP that outputs RGB. This MLP comprises four layers of 128 hidden units each. The Personal MLP, consisting of four layers of 128 hidden units, outputs both $\mathbf{\sigma}$ and color. Details on positional encoding, encoding viewing direction, and other aspects are in line with NeRF-W and are mentioned in the supplementary material. For DecentNeRF, we implement the same architecture on the user device, which we simulate using the open-source Flower library \cite{beutel2020flower}. This implementation includes the secure aggregation protocol of SecAgg+ \cite{bonawitz2017practical}, a feature of Flower. The FedNeRF implementation is akin to DecentNeRF but omits the Personal MLP, appearance embedding, secure aggregation, and learned weighted averaging.

During training, we sample 64 points for coarse and 64 for fine part of the network while for inference we sample 128 fine samples for all implementations. Models are trained with Adam for the same number of total iterations (sum of all user iterations for decentralized) for NeRF-W and DecentNeRF while FedNeRF is trained for lower rounds as the validation loss doesn't improve beyond certain rounds.

\section{Model Extraction Attacks and Defenses}
\label{sec:limiations_supp}
There are model-extraction attacks that attempt to recover individual weights of the model reported by any client \cite{truong2021data,sanyal2022towards} even if the weights were to be securely aggregated to compute the averaged weight. These attacks have been studied in the context of federated learning along with other attacks such as backdoor attacks \cite{bagdasaryan2020backdoor} for adversarially poisoning a federated learning system. Similarly, there have been several defenses based on differential privacy, such as the PrivUnit mechanism \cite{bhowmick2018protection} to prevent such attacks. The study of federated learning systems in the context of various such attacks is out of scope of this paper. The contributions of our paper hold independently to help enable a real-world vision application. That said, our method is in fact forward-compatible with the PrivUnit defense to prevent reconstruction of client weights. 

\section{Dataset Details}
\label{sec:supp_dataset}
\noindent \textbf{Phototourism dataset} Even though the scenes from the phototourism dataset vary in number of images we only use the first 200 images for all approaches since for our decentralized approaches we need to simulate multiple clients and a single machine. The real implementation of our decentralized wouldn't have this restriction and can learn on more than 200 images.

\section{DecentNeRF pseudocode}

\begin{algorithm}
\caption{DecentNeRF algorithm. Data transfers are marked by \textcolor{blue}{*}.\zt{fix naming convention, random initialization of wts, add in parallel and secure compute, refer to sections}}
\label{alg:panda}
\begin{algorithmic}[1]
\REQUIRE Hyperparameters: \\
Weighted Averaging Learning Rate $\eta$, \\
Number of merge rounds $M$, \\
Number of training epochs per merge $\Gamma$.
\STATE $\{g^{(0)}, p^{(0)}\}$ are initial Shared and Public MLP weights
\STATE $\alpha^{(0)} \rightarrow \{\alpha_1,\alpha_2,\ldots,\alpha_K\}$ are initial client contributions
\STATE Distribute $\{g^{(0)}, p^{(0)}\}$ to all clients $k = 1, \ldots, K$ \textcolor{blue}{*}
\FOR{merge round $m = 1$ to $M$}
    \FOR{client $k = 1$ to $K$ in Parallel}  %\COMMENT{parallel loop}
        \STATE $g^{(m-1)}$ is received from the server \textcolor{blue}{*}
        % \IF {$m=1$}
        %     \STATE $p^{(m-1)}$ is received from the server \textcolor{blue}{*}
        % \ENDIF
        \IF{$m > 1$}
            \STATE freeze $\{g_k^{(m-1)}, p_k^{(m-1)}\}$
            \STATE $\frac{\partial L_k}{\partial g_k^{(m-1)}} \leftarrow \text{\emph{Calc. Gradients}}$
            \STATE $\frac{\partial L_k}{\partial g_k^{(m-1)}}$ transmitted to the server \textcolor{blue}{*}
            \STATE $\sum \frac{\partial L_k}{\partial \mathbf{g}^{(m-1)}}$ is recieved from the server \textcolor{blue}{*}
            \STATE $\alpha_k^{(m)} \leftarrow \text{Alpha Update}(\left\{\frac{\partial L_k}{\partial g_k^{(m-1)}}, g_k^{(m-1)},\eta\right\})$
        \ENDIF
        \STATE $\{g_k^{(m)}, p_k^{(m)}\} \leftarrow \text{NeRF}(g_k^{(m-1)}, p_k^{(m-1)}, \Gamma)$
        \STATE $\alpha_k^{(m)} \times g_k^{(m)}$ is transmitted to the server \textcolor{blue}{*}
    \ENDFOR

    \FOR{ server in Parallel }
   
        \STATE $g^{(m)} \leftarrow \text{Secure Aggregation}( \{ \alpha_k \times g_k \} _{k=1,\ldots,K}^{(m)})$
        \STATE $g^{(m)}$ is transmitted to the clients \textcolor{blue}{*}
        \STATE $\sum \frac{\partial L_k}{\partial \mathbf{g}^{(m-1)}} \leftarrow \text{Secure Aggregation}(\{ \frac{\partial L_k}{\partial g_k^{(m-1)}}\}_{k=1,\ldots,K})$
        \STATE  $\sum \frac{\partial L_k}{\partial \mathbf{g}^{(m-1)}}$ is transmitted to the clients \textcolor{blue}{*}        
    \ENDFOR
\ENDFOR
\RETURN $g^{(M)}$
\end{algorithmic}
\end{algorithm}

% g_{k=1,\ldots,K}^{(m)

% \section{NeRF-W Preliminaries}
% \subsection{NeRF}\label{supp:nerf_pipeline}

% Our Global MLPs (\mathbf{G}) takes as input a 3D position $\mathbf{x} = (x,y,z)$ and viewing direction $\mathbf{d} = (\theta, \phi)$, and produce an output density $\sigma$ and color $\mathbf{c} = (r,g,b)$. To compute the color of a single pixel, NeRF approximates the volumetric rendering integral using a quadrature (Eq. 1) to yield Eq. 1 to Eq. 4:

% % 

% \subsection{NeRF in the Wild (NeRF-W)}\label{supp:nerfw_details}
