# Supplementary material for: DecentNeRFs: Decentralized Neural Radiance Fields from Crowdsourced Images
Source: arXiv:2403.13199 source file (2024-03-28)
Supplement: Supplementary file 2 [file results_supp.tex]

\section{Results}
\label{sec:results}
\subsection{Datasets}
\label{sec:datasets}
\textbf{Private Blender Dataset}: Since there are no datasets that exist for privacy evaluations on NeRF we generate our own dataset. We do it by adding personal content in the form of lego people to the original synthetic dataset introduced in \cite{nerf}. Representative views from the novel dataset are shown in the supplementary.

Each scene in this dataset has 100 views distributed between 20 users covering the full 360 yaw changes rotation. Hence each user has 5 images on their device distributed in a non-IID partitioning in terms of yaw angle spanning 18 degrees. In terms of lego people occlusion, we add 6 people per view where 1 person remains static within each users' views while the rest of them move around. This is to simulate real world scenarios like people taking images in front of a famous landmark, where the subject is static while the crowd moves around. While the subject would be static wrt to the user, PANDA would still be able to figure out that it's personal content. All images are rendered at 800x800 pixels and also provided with masks for privacy evaluation wherever the personal content i.e. people exist. 

\textbf{Phototourism Dataset:} We do image reconstruction evaluation on 3 scenes evaluated in \cite{martin2021nerf,chen2022hallucinated,yang2023cross} for the problem of novel-view synthesis
from unconstrained image collections: Bradenburg Gate (763), Trevi Fountain(1689) and Sacre Couer(830) \cite{phototourism}. We simulate 20 users each having 10 images. In total we train on 200 images downsampled for a factor of 2, for all PANDA and baseline experiments for a fair evaluation. Downsampling helps in avoiding OOM issues while simulating users, and we use only a subset of images of the total available because it's expensive to simulate multiple users in terms of number of GPU requirements. This is just a simulation constraint as the real-world deployment of our approach doesn't require the any central training.

\subsection{Experimental Details}
\textbf{Baselines}
We compare PANDA with a Centralized Privacy-Agnostic approach (NeRF-W\cite{martin2021nerf}) and a Decentralized Privacy-Agnostic approach. (FedNerF\cite{holden2023federated}). For PANDA, we run two ablations, PANDA(-P) without the Personal MLP, and PANDA(-L) without the learned weighted averaging. When we say PANDA we mean our full suite of features unless mentioned otherwise.

\textbf{Implementation details}
We use a PyTorch implementation of NeRF-W \cite{nerf_pl_nerfw} for centralized evaluation, which is a variant of vanilla NeRF \cite{nerf}. As shown in Figure~\ref{fig:method}, the Global Radiance Field $\mathbf{G}$, consists of eight layers with 256 hidden units each, followed by an MLP that outputs RGB. This MLP comprises four layers of 128 hidden units each. The Personal MLP, consisting of four layers of 128 hidden units, outputs both $\mathbf{\sigma}$ and color. Details on positional encoding, encoding viewing direction, and other aspects are in line with NeRF-W and are mentioned in the supplementary material. For PANDA, we implement the same architecture on the user device, which we simulate using the open-source Flower library \cite{beutel2020flower}. This implementation includes the secure aggregation protocol of SecAgg \cite{bonawitz2017practical}, a feature of Flower. The FedNeRF implementation is akin to PANDA but omits the Personal MLP, appearance embedding, secure aggregation, and learned weighted averaging.

During training, we sample 64 points for coarse and 64 for fine part of the network while for inference we sample 128 fine samples for all implementations. Models are trained with Adam for the same number of total iterations (sum of all user iterations for decentralized) for all approaches.

\subsection{Evaluation Metrics and Protocols}
We present the evaluation metrics for privacy, utility, and decentralization.

\textbf{Blender Photorealism results}: We use the same metrics of PSNR, SSIM and LPIPS as described in all NeRF evaluations \cite{nerf,holden2023federated} on the Global MLP Renderings for all approaches.

\textbf{Blender privacy evaluation}: Central computing (NeRFW) is considered non-private. We render views for the server-accessible MLPs which would be users' Global MLPs for FedNeRF and Server Global (securely aggregated) MLP for PANDA.  Our private Blender dataset comes with masks for all images denoting the areas of private scene content. We calculate SSIM and PSNR on the masked region on rendered images of all the MLPs for all the training views and all rounds for proper privacy evaluation. Reconstruction error is a loss used by most empirical evaluations of privacy \cite{singh2021disco,pittaluga2019revealing} in the absence of formal guarantees.

\textbf{Phototourism evaluation} We use the same protocol as in \cite{martin2021nerf} for fitting the appearance of the left half of the validation images and evaluating on the right half for PANDA and NeRFW using SSIM, PSNR, and SSIM.

\textbf{Decentralization}: We calculate server and per-user compute in terms of FLOPs for all approaches. For users it is NeRF training compute, while the server compute includes aggregation (for PANDA and FedNeRF) and reconstruction cost for secure aggregation and user weight update (for PANDA) as well. We provide a detailed analysis in the supplementary. To do a fair comparison we use the FLOPs computation from the SOTA NeRF training \cite{muller2022instant}. 

%------------------------------------
\subsection{Results on Private Blender Dataset}
\

% \begin{table}[h!]
%     \centering
%     \begin{tabular}{c|ccc|cc|ccc|cc}
%      & \multicolumn{5}{|c|}{Lego} & \multicolumn{5}{|c|}{Ship} \\
%      \hline 
     
%      & PSNR \uparrow &  SSIM \uparrow & LPIPS \downarrow 
%     \end{tabular}
%     \caption{Caption}
%     \label{tab:blender_baseline}
% \end{table}

% ---- dump google sheet copy/paste here
% \begin{scontents}[write-out=data.csv]
% 	Lego					Ship				
% 	Utility			Privacy	Decentralization	Utility			Privacy	Decentralization 
% 	PSNR\uparrow	SSIM\uparrow	LPIPS\downarrow	PSNR\downarrow SSIM\uparrow	Server (Flops)\downarrow PSNR\uparrow	SSIM\uparrow	LPIPS\downarrow	SSIM\downarrow	Server FLOPs\downarrow
% NeRF-W \cite{martin2021nerf}	\textcolor{blue}{27.09}	\textcolor{blue}{0.934}	\textcolor{blue}{0.0513}	0	20 M	\textcolor{blue}{26.35}	\textcolor{blue}{0.8661}	\textcolor{blue}{0.1765}	1	20 M
% FedNeRF \cite{holden2023federated}	17.7	0.858	0.2003	\textcolor{BurntOrange}{0.08}	\textcolor{blue}{1K}	20.92	0.8281	0.2368	\textcolor{BurntOrange}{0.92}	\textcolor{blue}{1K}
% PANDA (ours)	\textcolor{BurntOrange}{26.25}	\textcolor{BurntOrange}{0.92}	\textcolor{BurntOrange}{0.0652}	\textcolor{blue}{0.2}	\textcolor{BurntOrange}{10K}	\textcolor{BurntOrange}{24.58}	\textcolor{BurntOrange}{0.8554}	\textcolor{BurntOrange}{0.1901}	\textcolor{blue}{0.23}	\textcolor{BurntOrange}{10K}
% \end{scontents}

\begin{scontents}[write-out=data.csv]
	Lego						Ship					
	Utility			Privacy		Decentralization	Utility			Privacy		Decentralization
	PSNR\uparrow	SSIM\uparrow	LPIPS\downarrow	PSNR\downarrow	SSIM\downarrow	Server FLOPs\downarrow	PSNR\uparrow	SSIM\uparrow	LPIPS\downarrow	PSNR\downarrow	SSIM\downarrow	Server FLOPs\downarrow
NeRF-W 	\textcolor{Blue}{27.09}	\textcolor{Blue}{0.934}	\textcolor{Blue}{0.0513}	\infty	0	130 T	\textcolor{Blue}{26.35}	\textcolor{Blue}{0.8661}	\textcolor{Blue}{0.1765}	\infty	0	$\approx$ 220T
FedNeRF	17.7	0.858	0.2003	26.06	0.81	0.6 B	20.92	0.8281	0.2368	27.21	0.82	$\approx$ 1 B
PANDA 	\textcolor{BurntOrange}{26.25}	\textcolor{BurntOrange}{0.92}	\textcolor{BurntOrange}{0.0652}	14.59	0.62	4.8 B	\textcolor{BurntOrange}{24.58}	\textcolor{BurntOrange}{0.8554}	\textcolor{BurntOrange}{0.1901}	13.79	0.61	$\approx$ 8 B
\end{scontents}



% NeRF-W (centralized privacy-agnostic) FedNeRF (decentralized privacy-agnostic) PANDA (decentralized privacy-aware)

\begin{table*}[ht]
\centering 
\scalebox{0.77}{{\begin{tabularx}{\textwidth}{l|ccc|cc|c|ccc|cc|c}
\input{|python script.py}
\end{tabularx}}}
\caption{\textbf{Quantitative results on Private Blender dataset}:
Best and second best results for utility are highlighted in blue and orange respectively. A privacy-agnostic centralized approach \cite{martin2021nerf} achieves the best utility performance while using ~\textbf{$10^5$} more server compute than other approaches. FedNerf \cite{holden2023federated} even though it only is 8x server compute cheaper than PANDA and performs poorly on utility metrics and leaks out the most private details as reference by the high SSIM an PSNR numbers. In contrast, PANDA obtains comparable utility to centralized approaches, is the most private, and has server computation several orders of magnitude lower than the centralized approach. Number of training rounds is different for FedNeRF and PANDA. }
\end{table*}

\input{figures/fig4_blender_qualitative/fig4_blender_qualitative}
\input{figures/blender_privacy/blender_privacy}
\zt{\begin{itemize}
    \item Static to the user while Transient to the Global Model
    \item Public Private improvement in learning time
\end{itemize}}

\subsection{Results on Phototourism}
\input{figures/fig5_photo_qualitative/fig5_v0}

% \begin{table}[h!]
%     \centering
%     \begin{tabular}{c|ccc|cc|ccc|cc}
%      & \multicolumn{5}{|c|}{Lego} & \multicolumn{5}{|c|}{Ship} \\
%      \hline 
     
%      & PSNR \uparrow &  SSIM \uparrow & LPIPS \downarrow 
%     \end{tabular}
%     \caption{Caption}
%     \label{tab:blender_baseline}
% \end{table}

% ---- dump google sheet copy/paste here
\begin{scontents}[write-out=data2.csv]
	Bradenburg Gate			Trevi Fountain			Sacre Coeur		
	PSNR\uparrow	SSIM\uparrow	LPIPS\downarrow	PSNR\uparrow	SSIM\uparrow	LPIPS\downarrow	PSNR\uparrow	SSIM\uparrow	LPIPS\downarrow
NeRF-W \cite{martin2021nerf}	\textcolor{blue}{25.18}	\textcolor{blue}{0.901}	\textcolor{blue}{0.1927}	\textcolor{blue}{21.49}	\textcolor{blue}{0.7206}	\textcolor{blue}{0.2866}	\textcolor{blue}{20.58}	\textcolor{blue}{0.7835}	\textcolor{blue}{0.2305}
FedNeRF \cite{holden2023federated}	18.92	0.8158	0.3528	16.55	0.5774	0.4352	15.41	0.6555	0.4072
PANDA(A)	23.61	0.8535	0.329	20.04	0.6439	0.5261	18.82	0.6777	0.3874
PANDA	\textcolor{BurntOrange}{24.62}	\textcolor{BurntOrange}{0.8802}	\textcolor{BurntOrange}{0.2571}	\textcolor{BurntOrange}{20.61}	\textcolor{BurntOrange}{0.6501}	\textcolor{BurntOrange}{0.3963	} \textcolor{BurntOrange}{19.22}	\textcolor{BurntOrange}{0.7259}	\textcolor{BurntOrange}{0.3126}
\end{scontents}



\begin{table*}[h!]
\centering
\label{tab:photo_qual}
%\resizebox{\linewidth}{!}
{\scalebox{0.74}{\begin{tabularx}{\textwidth}{l|ccc|ccc|ccc}
\input{|python script.py}
\end{tabularx}}}
\caption{\textbf{Quantitative reconstruction performance on Phototoursim dataset\cite{snavely2006photo} for NeRF-W, FedNeRF, and PANDA ablations}: Best and second best results are highlighted in blue and orange respectively. As expected, privacy-agnostic centralized NeRF-W \cite{martin2021nerf} performs best across all metrics, followed closely by PANDA. This demonstrates our privacy-aware decentralized approach (PANDA) is effective for real-world datasets compared to other privacy-agnostic decentralized approaches \cite{holden2023federated} }
\end{table*}

% \begin{table*}[]
% \centering
% \begin{tabular}{|l|lll|lll|lll|}
% \hline
% Method   & \multicolumn{3}{c|}{Bradenberg Gate}                & \multicolumn{3}{c|}{Trevi Fountain}                 & \multicolumn{3}{c|}{Sacre Coeur}                    \\ \hline
%  &
%   \multicolumn{1}{l|}{PSNR} &
%   \multicolumn{1}{l|}{SSIM} &
%   LPIPS &
%   \multicolumn{1}{l|}{PSNR} &
%   \multicolumn{1}{l|}{SSIM} &
%   LPIPS &
%   \multicolumn{1}{l|}{PSNR} &
%   \multicolumn{1}{l|}{SSIM} &
%   LPIPS \\ \cline{2-10} 
% NeRF-W   & \multicolumn{1}{l|}{1} & \multicolumn{1}{l|}{1} & 2 & \multicolumn{1}{l|}{2} & \multicolumn{1}{l|}{3} & 3 & \multicolumn{1}{l|}{2} & \multicolumn{1}{l|}{3} & 3 \\
% FedNeRF  & \multicolumn{1}{l|}{2} & \multicolumn{1}{l|}{1} & 2 & \multicolumn{1}{l|}{2} & \multicolumn{1}{l|}{3} & 3 & \multicolumn{1}{l|}{2} & \multicolumn{1}{l|}{3} & 3 \\
% PANDA(A) & \multicolumn{1}{l|}{3} & \multicolumn{1}{l|}{1} & 2 & \multicolumn{1}{l|}{2} & \multicolumn{1}{l|}{3} & 3 & \multicolumn{1}{l|}{2} & \multicolumn{1}{l|}{3} & 3 \\
% PANDA    & \multicolumn{1}{l|}{3} & \multicolumn{1}{l|}{1} & 2 & \multicolumn{1}{l|}{2} & \multicolumn{1}{l|}{3} & 3 & \multicolumn{1}{l|}{2} & \multicolumn{1}{l|}{3} & 3\\
% \hline
% \end{tabular}
% \end{table*}

\subsection{Ablation on Smart Aggregation}
\input{figures/fig6_smart_aggregation/fig6_v0}
